# Supplementary material for: Efficient Real-world Image Super-Resolution Via Adaptive Directional Gradient Convolution
Source: arXiv:2405.07023 source file (2024-05-11)
Supplement: Supplementary file 1 [file supplementary.tex]

% % \clearpage
% \setcounter{page}{1}
% % \maketitlesupplementary
% % \onecolumn

% % \section{Rationale}
% % \label{sec:rationale}
% % % 
% % Having the supplementary compiled together with the main paper means that:
% % % 
% % \begin{itemize}
% % \item The supplementary can back-reference sections of the main paper, for example, we can refer to \cref{sec:intro};
% % \item The main paper can forward reference sub-sections within the supplementary explicitly (e.g. referring to a particular experiment); 
% % \item When submitted to arXiv, the supplementary will already included at the end of the paper.
% % \end{itemize}
% % % 
% % To split the supplementary pages from the main paper, you can use \href{https://support.apple.com/en-ca/guide/preview/prvw11793/mac#:~:text=Delete%20a%20page%20from%20a,or%20choose%20Edit%20%3E%20Delete).}{Preview (on macOS)}, \href{https://www.adobe.com/acrobat/how-to/delete-pages-from-pdf.html#:~:text=Choose%20%E2%80%9CTools%E2%80%9D%20%3E%20%E2%80%9COrganize,or%20pages%20from%20the%20file.}{Adobe Acrobat} (on all OSs), as well as \href{https://superuser.com/questions/517986/is-it-possible-to-delete-some-pages-of-a-pdf-document}{command line tools}.


% % \section{Adaptive Spatial Arrangement Perceiving for Real-world Image Super-Resolution (Supplementary Materials)}

% This supplementary document is organized as follows:

% 1. We provide \textbf{the statistical experiments on directional gradients}, as shown in section \ref{Statistical experiments on directional gradients}.


% 2. We provide more \textbf{details about the proposed DGConv}, as shown in section \ref{Details about the proposed DGConv}.

% 3. We provide more \textbf{details about the proposed equivalent transformation}, as shown in section \ref{Details about the proposed equivalent transformation}.

% 4. We provide more \textbf{details about the experimental environment}, as shown in section \ref{Details about the experimental environment}.


% 5. We provide \textbf{details about the evaluation of existing methods}, as shown in section \ref{Details about the evaluation of existing methods}.

% 6. We provide more \textbf{ablation studies on DGConv and DGPNet}, as shown in section \ref{More ablation studies}.


% 7. We provide more \textbf{details about the comparison with existing methods in Parameter and FLOPs}, as shown in section \ref{Detail about comparison with existing methods in Parameter and FLOPs}.

% 8. We provide \textbf{evidence of cost-free improvement of DGConv}, as shown in section \ref{The evidence of cost-free improvement of DGConv}.



% 9. We provide more \textbf{detail about qualitative experimental results}, as shown in section \ref{More detail about qualitative experimental results}.

% 10. We provide \textbf{the analysis of the kernel size of DGConv}, as shown in section \ref{Analysis of the kernel size of DGConv}.

% 11. We provide \textbf{reasons for using local mean in center-surrounding gradient and center-surrounding aggregation convolutions}, as shown in section \ref{Reasons for using local mean in center-surrounding gradient and center-surrounding aggregation convolutions}.

% 12. We provide \textbf{sample visualizations of our test data set}, as shown in section \ref{Sample visualizations of test data set}.

% 13. We provide \textbf{the feature visualization of proposed learnable convolutions}, as shown in section \ref{Feature visualization}.









% \section{Statistical experiments on directional gradients}
% \label{Statistical experiments on directional gradients}


% \begin{figure*}[h]
%     \centering
%     \includegraphics[width=1.0\linewidth]{Fig/t-snet-vis.png}
%     \caption{Statistical experiments on directional gradients}

%     \label{fig:sta}
% \end{figure*}

% In Fig 1 of the main text, we observe that during the imaging process, real LR images are often degraded by various degradation factors, such as blur, noise, and JPEG. At the same time, we can observe that there are significant directional gradient differences between these degradations. To further demonstrate the differences in directional gradients under different degradations, we conduct the following statistical experiment: We randomly select 100 patches from natural clear images and then add blur, noise, and JPEG degradations respectively, and directly through t-SNE statistics. We observe that patches with different degradation cues are coupled together, as shown in the blue points of Fig. \ref{fig:sta} (c). However, after extracting horizontal, vertical, and center-surrounding directional gradients of those patches, we observed that patches with different degradation cues can be significantly distinguished. This proves the differences in directional gradient distribution of different degradations and also proves that the three proposed gradients in horizontal, vertical, and center-surrounding directions can effectively distinguish different degradation types, facilitating the modeling of unified degradation representations of real LR images.






% \section{Details about the proposed DGConv}
% \label{Details about the proposed DGConv}
% First, we mark the learnable kernels in vanilla convolution, center-surrounding gradient convolution, center-surrounding aggregation convolution, horizontal gradient convolution, and vertical gradient convolution as ${\omega_{vc}}$, ${\omega_{csg}}$, ${\omega_{csa}}$, ${\omega_{hg}}$, and ${\omega_{vg}}$ respectively. Then, we mark that the output of vanilla convolution, center-surrounding gradient convolution, center-surrounding aggregation convolution, horizontal gradient convolution, and vertical gradient convolution as ${F_{vc}}(X)$, ${F_{csg}}(X)$, ${F_{csa}}(X)$, ${F_{hg}}(X)$, and ${F_{vg}}(X)$ respectively, as expressed in the following:

% \begin{equation}
%     {F_{vc}}(X) = \sum\limits_{i = 1}^9 {{\omega_{vc_i}}}  \cdot {x_i}.\\
% \end{equation}


% \begin{equation}
% {F_{csg}}(X) = \sum\limits_{i = 1}^9 {{\omega_{csg_i}}}  \cdot \left( {{x_i} - \frac{1}{9}{{\sum\limits_{i = 1}^9 {{x_{_i}}} }}} \right).\\
% \end{equation}


% \begin{equation}
% {F_{csa}}(X) = \sum\limits_{i = 1}^9 {{\omega_{csa_i}}}  \cdot \left( {{x_i} + \frac{1}{9}{{\sum\limits_{i = 1}^9 {{x_{_i}}} }}} \right).\\
% \end{equation}


% \begin{equation}
% \begin{array}{l}


% {F_{hg}}(X) = {\omega_{hg_1}} \cdot \left( {{x_1} - {x_3}} \right) + {\omega_{hg_2}} \cdot 0 + {\omega_{hg_3}} \cdot \left( {{x_3} - {x_1}} \right)\\
% \;\;\;\;\;\;\;\;\;\;\; + {\omega_{hg_4}} \cdot \left( {{x_4} - {x_6}} \right) + {\omega_{hg_5}} \cdot 0 + {\omega_{hg_6}} \cdot \left( {{x_6} - {x_4}} \right)\\
% \;\;\;\;\;\;\;\;\;\;\; + {\omega_{hg_7}} \cdot \left( {{x_7} - {x_9}} \right) + {\omega_{hg_8}} \cdot 0 + {\omega_{hg_9}} \cdot \left( {{x_9} - {x_7}} \right).\\
% \\

% \end{array}
% \end{equation}


% \begin{equation}
% \begin{array}{l}

% {F_{vg}}(X) = {\omega_{vg_1}} \cdot \left( {{x_1} - {x_7}} \right) + {\omega_{vg_2}} \cdot \left( {{x_2} - {x_8}} \right) + {\omega_{vg_3}}\cdot \left( {{x_3} - {x_9}} \right)\\
% \;\;\;\;\;\;\;\;\;\;\; \;\; \;+ {\omega_{vg_4}} \cdot 0\;\;\;\;\;\;\;\;\;\;\; + {{\omega_{vg_5}} \cdot 0\;\;\;\;\;\;\;\;\;\;\;\; + {\omega_{vg_6}} \cdot 0\\
% \;\;\;\;\;\;\;\;\;\;\; + {\omega_{vg_7}} \cdot \left( {{x_7} - {x_1}} \right) + {\omega_{vg_8}} \cdot \left( {{x_8} - {x_2}} \right) + {\omega_{vg_8}} \cdot \left( {{x_9} - {x_3}} \right).
% \end{array}
% \end{equation}


% Then, we concat kernels of all branches as input to learnable linear.

% \begin{equation}
% w_{all}  = cat(\omega_{vc}, w_{csg}, w_{csa}, w_{hg}, w_{vg}).
% \end{equation}

% We use five learnable $linear$ (\emph{i.e.}, torch.nn.Linear in pytorch code) layers to learn each branch's balance factor $\alpha$. 

% \begin{equation}
% \alpha_{vc}=linear_{vc}(\omega_{all}).
% \end{equation}

% \begin{equation}
% \alpha_{csg}=linear_{csg}(\omega_{all}).
% \end{equation}

% \begin{equation}
% \alpha_{csa}=linear_{csa}(\omega_{all}).
% \end{equation}

% \begin{equation}
% \alpha_{hg}=linear_{hg}(\omega_{all}).
% \end{equation}

% \begin{equation}
% \alpha_{vg}=linear_{vg}(\omega_{all}).
% \end{equation}

% Finally, we add all branches together, and the proposed DGConv ${F_{dg}}(X)$ is shown in the following formula:

% \begin{equation}
% F_{dg}(X) = {\alpha_{vc}} \cdot {F_{vc}}(X) + {\alpha_{csg}} \cdot {F_{csg}}(X) + {\alpha_{csa}} \cdot {F_{csa}}(X)+ {\alpha_{hg}} \cdot {F_{hg}}(X) + {\alpha_{vg}} \cdot {F_{vg}}(X).
% \end{equation}






% \section{Details about the proposed equivalent transformation}
% \label{Details about the proposed equivalent transformation}
% After training, to improve the efficiency of the proposed DGConv, we propose an equivalent transformation for DGConv, which can fuse DGConv to a single VC, thus significantly reducing the calculation cost of DGConv. As a result, our equivalent transformation makes DGConv enhance existing VC representation capacity without introducing additional computational costs during inferencing. After using the proposed equivalent transformation, the model complexity of DGConv is the same as that of VC during inferencing. Specifically, we first equate the four proposed novel convolutions to VC-style kernels. 

% \subsection{Equivalent transformation for learnable center-surrounding gradient convolution}

% The equivalent transformation for learnable center-surrounding gradient convolution is as follows:

% \begin{equation}
% {F_{csg}(X)} = \sum\limits_{i = 1}^9 {{\omega_{csg_{i}}}}  \cdot \left( {{x_i} - \frac{1}{9}{{\sum\limits_{i = 1}^9 {{x_{_i}}} }}} \right).
% \end{equation}
% We expand the above equation and combine the coefficients of ${x_i}$, and get the following equation:

% \begin{equation}
% \begin{array}{l}
% \begin{array}{l}
% {F_{csg}(X)} = \sum\limits_{i = 1}^9 {{\omega_{csg_i}}}  \cdot \left( {{x_i} - \frac{{\sum\limits_{i = 1}^9 {{x_{_i}}} }}{9}} \right)\\
%  \;\;\;\;\;\;\;\;\;\; \;\;= {\omega_{csg}}_{_1} \cdot \left( {{x_1} - \frac{{\left( {{x_1} + {x_2} + {x_3} + {x_4} + {x_5} + {x_6} + {x_7} + {x_8} + {x_9}} \right)}}{9}} \right) + {\omega_{csg}}_{_2} \cdot \left( {{x_2} - \frac{{\left( {{x_1} + {x_2} + {x_3} + {x_4} + {x_5} + {x_6} + {x_7} + {x_8} + {x_9}} \right)}}{9}} \right)\\ 
%  \;\;\;\;\;\;\;\;\;\; \;\; ... + {\omega_{csg}}_{_9} \cdot \left( {{x_9} - \frac{{\left( {{x_1} + {x_2} + {x_3} + {x_4} + {x_5} + {x_6} + {x_7} + {x_8} + {x_9}} \right)}}{9}} \right)\\
%   \;\;\;\;\;\;\;\;\;\; \;\;
%  = {x_1} \cdot \left( {{\omega_{csg}}_{_1} - \frac{{\left( {{\omega_{csg}}_{_1} + {\omega_{csg}}_{_2} + {\omega_{csg}}_{_3} + {\omega_{csg}}_{_4} + {\omega_{csg}}_{_5} + {\omega_{csg}}_{_6} + {\omega_{csg}}_{_7} + {\omega_{csg}}_{_8} + {\omega_{csg}}_{_9}} \right)}}{9}} \right) + ...\\
%   \;\;\;\;\;\;\;\;\;\; \;\;
%  + {x_9} \cdot \left( {{\omega_{csg}}_{_9} - \frac{{\left( {{\omega_{csg}}_{_1} + {\omega_{csg}}_{_2} + {\omega_{csg}}_{_3} + {\omega_{csg}}_{_4} + {\omega_{csg}}_{_5} + {\omega_{csg}}_{_6} + {\omega_{csg}}_{_7} + {\omega_{csg}}_{_8} + {\omega_{csg}}_{_9}} \right)}}{9}} \right)\\
%   \;\;\;\;\;\;\;\;\;\; \;\;
%  = \sum\limits_{i = 1}^9 {\left( {{\omega_{csg_{i}}} - \frac{{\sum\limits_{i = 1}^9 {{\omega_{csg_{i}}}} }}{9}} \right)}  \cdot \left( {{x_i}} \right).
% \end{array}
% \end{array}
% \label{supple_lap}
% \end{equation}



% \subsection{Equivalent transformation for learnable center-surrounding aggregation convolution}

% In the same way, we can get the equivalent transformation for learnable center-surrounding aggregation convolution, as follows:

% \begin{equation}
% \begin{array}{l}
% \begin{array}{l}
% {F_{csa}(X)}= \sum\limits_{i = 1}^9 {{\omega_{csa_i}}}  \cdot \left( {{x_i} + \frac{{\sum\limits_{i = 1}^9 {{x_{_i}}} }}{9}} \right)\\
%  \;\;\;\;\;\;\;\;\;\; \;\;= {\omega_{csa}}_{_1} \cdot \left( {{x_1} + \frac{{\left( {{x_1} + {x_2} + {x_3} + {x_4} + {x_5} + {x_6} + {x_7} + {x_8} + {x_9}} \right)}}{9}} \right) + {\omega_{csa}}_{_2} \cdot \left( {{x_2} + \frac{{\left( {{x_1} + {x_2} + {x_3} + {x_4} + {x_5} + {x_6} + {x_7} + {x_8} + {x_9}} \right)}}{9}} \right)\\ 
%  \;\;\;\;\;\;\;\;\;\; \;\; ... + {\omega_{csa}}_{_9} \cdot \left( {{x_9} + \frac{{\left( {{x_1} + {x_2} + {x_3} + {x_4} + {x_5} + {x_6} + {x_7} + {x_8} + {x_9}} \right)}}{9}} \right)\\
%   \;\;\;\;\;\;\;\;\;\; \;\;
%  = {x_1} \cdot \left( {{\omega_{csa}}_{_1} + \frac{{\left( {{\omega_{csa}}_{_1} + {\omega_{csa}}_{_2} + {\omega_{csa}}_{_3} + {\omega_{csa}}_{_4} + {\omega_{csa}}_{_5} + {\omega_{csa}}_{_6} + {\omega_{csa}}_{_7} + {\omega_{csa}}_{_8} + {\omega_{csa}}_{_9}} \right)}}{9}} \right) + ...\\
%   \;\;\;\;\;\;\;\;\;\; \;\;
%  + {x_9} \cdot \left( {{\omega_{csa}}_{_9} + \frac{{\left( {{\omega_{csa}}_{_1} + {\omega_{csa}}_{_2} + {\omega_{csa}}_{_3} + {\omega_{csa}}_{_4} + {\omega_{csa}}_{_5} + {\omega_{csa}}_{_6} + {\omega_{csa}}_{_7} + {\omega_{csa}}_{_8} + {\omega_{csa}}_{_9}} \right)}}{9}} \right)\\
%   \;\;\;\;\;\;\;\;\;\; \;\;
%  = \sum\limits_{i = 1}^9 {\left( {{\omega_{csa_{i}}} + \frac{{\sum\limits_{i = 1}^9 {{\omega_{csa_{i}}}} }}{9}} \right)}  \cdot \left( {{x_i}} \right).
% \end{array}
% \end{array}
% \label{supple_csa}
% \end{equation}


% \subsection{Equivalent transformation for learnable horizontal gradient convolution}

% The equivalent transformation for learnable horizontal gradient convolution is as follows:

% \begin{equation}
% \begin{array}{l}
% {F_{hg}}(X) = {\omega_{hg}}_{_1} \cdot \left( {{x_1} - {x_3}} \right) + {\omega_{hg}}_{_2} \cdot 0 + {\omega_{hg}}_{_3} \cdot \left( {{x_3} - {x_1}} \right) + {\omega_{hg}}_{_4} \cdot \left( {{x_4} - {x_6}} \right)\\
%  + {\omega_{hg}}_{_5} \cdot 0 + {\omega_{hg}}_{_6} \cdot \left( {{x_6} - {x_4}} \right) + {\omega_{hg}}_{_7} \cdot \left( {{x_7} - {x_9}} \right) + {\omega_{hg}}_{_8} \cdot 0 + {\omega_{hg}}_{_9} \cdot \left( {{x_9} - {x_7}} \right)\\
%  = {x_1} \cdot \left( {{\omega_{hg}}_{_1} - {\omega_{hg}}_{_3}} \right) + {x_2} \cdot 0 + {x_3} \cdot \left( {{\omega_{hg}}_{_3} - {\omega_{hg}}_{_1}} \right) + {x_4} \cdot \left( {{\omega_{hg}}_{_4} - {\omega_{hg}}_{_6}} \right)\\
%  + {x_5} \cdot 0 + {x_6} \cdot \left( {{\omega_{hg}}_{_6} - {\omega_{hg}}_{_4}} \right) + {x_7} \cdot \left( {{\omega_{hg}}_{_7} - {\omega_{hg}}_{_9}} \right) + {x_8} \cdot 0 + {x_9} \cdot \left( {{\omega_{hg}}_{_9} - {\omega_{hg}}_{_7}} \right).
% \end{array}
% \label{hg}
% \end{equation}


% \subsection{Equivalent transformation for learnable vertical gradient convolution}

% The equivalent transformation for learnable vertical gradient convolution is as follows:

% \begin{equation}
% \begin{array}{l}
% {F_{vg}}(X) = {\omega_{vg}}_{_1} \cdot \left( {{x_1} - {x_7}} \right) + {\omega_{vg}}_{_2} \cdot \left( {{x_2} - {x_8}} \right) + {\omega_{vg}}_{_3} \cdot \left( {{x_3} - {x_7}} \right) + {\omega_{vg}}_{_4} \cdot 0 + {\omega_{vg}}_{_5} \cdot 0\\
%  + {\omega_{vg}}_{_6} \cdot 0 + {\omega_{vg}}_{_7} \cdot \left( {{x_7} - {x_1}} \right) + {\omega_{vg}}_{_8} \cdot \left( {{x_8} - {x_2}} \right) + {\omega_{vg}}_{_9} \cdot \left( {{x_9} - {x_3}} \right)\\
%  = {x_1} \cdot \left( {{\omega_{vg}}_{_1} - {\omega_{vg}}_{_7}} \right) + {x_2} \cdot \left( {{\omega_{vg}}_{_2} - {\omega_{vg}}_{_8}} \right) + {x_3} \cdot \left( {{\omega_{vg}}_{_3} - {\omega_{vg}}_{_7}} \right) + {x_4} \cdot 0 + {x_5} \cdot 0\\
%  + {x_5} \cdot 0 + {x_7} \cdot \left( {{\omega_{vg}}_{_7} - {\omega_{vg}}_{_1}} \right) + {x_8} \cdot \left( {{\omega_{vg}}_{_8} - {\omega_{vg}}_{_2}} \right) + {x_9} \cdot \left( {{\omega_{vg}}_{_9} - {\omega_{vg}}_3} \right).
% \end{array}
% \label{vg}
% \end{equation}
% Then, we need to translate the above to a VC-style kernel further. For Eq. \ref{supple_lap}, we can translate Eq. \ref{supple_lap} to follows:

% \begin{equation}
% \begin{array}{l}
% {F_{csg}(X)} = \sum\limits_{i = 1}^9 {{\omega^*}_{la{p_i}}}  \cdot \left( {{x_i}} \right)\\
% {\omega^*}_{la{p_i}} = \left( {{\omega_{la{p_i}}} - \frac{1}{9}{\sum\limits_{i = 1}^9 {{\omega_{la{p_i}}}} }} \right).
% \end{array}
% \end{equation}
% For Eq. \ref{supple_csa}, we can translate Eq. \ref{supple_csa} to follows:
% \begin{equation}
% \begin{array}{l}
% {F_{csa}(X)}= \sum\limits_{i = 1}^9 {{\omega^*}_{ala{p_i}}}  \cdot \left( {{x_i}} \right)\\
% {\omega^*}_{ala{p_i}} = \left( {{\omega_{ala{p_i}}} + \frac{1}{9}{\sum\limits_{i = 1}^9 {{\omega_{ala{p_i}}}} }}} \right).
% \end{array}
% \end{equation}
% For Eq. \ref{hg}, we can translate Eq. \ref{hg} to follows:
% \begin{equation}
% \begin{array}{l}
% {F_{hg}}(X) =  \sum\limits_{i = 1}^9 {{\omega^*}_{hg}}  \cdot \left( {{x_i}} \right)\\
% {\omega^*}_{hg} = \{ \left( {{\omega_{hg}}_{_1} - {\omega_{hg}}_{_3}} \right),0,\left( {{\omega_{hg}}_{_3} - {\omega_{hg}}_{_1}} \right),\\
% \; \; \; \; \; \; \; \; \; \; \; \; \;\; \; \; \ \left( {{\omega_{hg}}_{_4} - {\omega_{hg}}_{_7}} \right),0,\left( {{\omega_{hg}}_{_7} - {\omega_{hg}}_{_3}} \right)

% \\ \; \; \; \; \; \; \; \; \; \; \; \; \;\; \; \; \;
% \left( {{\omega_{hg}}_{_7} - {\omega_{hg}}_{_9}} \right),0,\left( {{\omega_{hg}}_{_9} - {\omega_{hg}}_{_7}} \right)\}. 
% \end{array}
% \end{equation}
% For Eq. \ref{vg}, we can translate Eq. \ref{vg} to follows:

% \begin{equation}
% \begin{array}{l}
% {F_{vg}}(X) =  \sum\limits_{i = 1}^9 {{\omega^*}_{vg}}  \cdot \left( {{x_i}} \right)\\
% {\omega^*}_{vg} = \{ \left( {{\omega_{vg}}_{_1} - {\omega_{vg}}_{_7}} \right), \left( {{\omega_{vg}}_{_2} - {\omega_{vg}}_{_8}} \right),\left( {{\omega_{vg}}_{_3} - {\omega_{vg}}_{_9}} \right),\\
% \; \; \; \; \; \; \; \; \; \; \; \; \;\; \; \; \ \; \; \; \; \; \; \; \; \; \; \; \; \;\; \; \;0,
% \; \; \; \; \; \; \; \; \;  \; \; \; \; \; \; \; \; \; \; \; \; \; \;\; \; \;0,
% \; \; \; \; \; \; \; \; \; \; \; \; \; \; \; \; \; \; \; \; \; \; \; \;\; \; \;0

% \\ \; \; \; \; \; \; \; \; \; \; \; \; \;\; \; \; \;
% \left( {{\omega_{vg}}_{_7} - {\omega_{vg}}_{_1}} \right),\left( {{\omega_{vg}}_{_8} - {\omega_{vg}}_{_2}} \right),\left( {{\omega_{vg}}_{_9} - {\omega_{vg}}_{_3}} \right)\}.
% \end{array}
% \end{equation}
% Finally, we utilize the linearity of convolution and structure reparameterize \cite{ding2021repvgg} to fuse all kernels into a single final kernel ${\omega^*}_{f}$.

% \begin{equation}
% \begin{array}{l}
% {\omega^*}_f = {\alpha_{vc}} \cdot {\omega_{vc}} + {\alpha_{csg}} \cdot {\omega^*}_{lap} + {\alpha_{csa}} \cdot {\omega^*_{csa}}+ {\alpha_{hg}} \cdot {\omega^*}_{hg} + {\alpha_{vg}} \cdot {\omega^*}_{vg}.
% \end{array}
% \end{equation}
% To this end, we equate the proposed DGConv to a single VC during inferencing, which can improve the VC representation capacity without introducing computational costs.


% \begin{equation}
% \begin{array}{l}
% \begin{array}{*{20}{l}}
% {{F_{dg}}(X) = {\alpha_{vc}} \cdot {F_{vc}}(X) + {\alpha_{csg}} \cdot {F_{lap}}(X) + {\alpha_{csa}} \cdot {F_{csa}}}(X)+ {\alpha_{hg}} \cdot {F_{hg}}(X) + {\alpha_{vg}} \cdot {F_{vg}}}(X)
% \end{array}\\
% \;\;\;\;\;\;\;\;\;\;\;\;\;\;= \sum\limits_{i = 1}^9 {{\omega^*}_f}  \cdot {x_i}.
% \end{array}
% \end{equation}
% \section{Details about the experimental environment}
% \label{Details about the experimental environment}
% We perform our experiment on four NVIDIA RTX3090 (24G) GPUs at Pytorch \cite{paszke2019pytorch}. The CPU core is 32, the CPU memory is 163840 MB, and the GPU memory is 96 GB. The main package includes pytorch=1.13, opencv-python=4.6.0.66, pillow=9.0.1, numpy=1.21.5, scipy=1.7.3, and so on. More details will be shown in the open-source code.



% \section{Details about the evaluation of existing methods}
% \label{Details about the evaluation of existing methods}
% As shown in the main body, we compare our model with fifteen state-of-the-art Real-SR methods, including SRResNet \cite{SRResNet}, EDSR \cite{EDSR}, RRDB \cite{wang2018esrgan}, VDSR \cite{VDSR}, SwinIR \cite{Swinir}, HAT \cite{HAT}, DAN \cite{DAN}, IKC \cite{IKC}, Real-ESRGAN\cite{wang2021real}, BSRGAN \cite{BSRGAN}, ESRGAN \cite{wang2018esrgan}, ESRGAN-FS \cite{ESRGAN-FS}, GFSNet \cite{GFSNet}, DASR \cite{DASR}, HGGT \cite{HGGT}. Following \cite{BSRGAN}.

% For widely-used image super-resolution (SR) baselines, we retrain them in the same way as our method for a fair comparison, including SRResNet, EDSR, RRDB, VDSR, SwinIR, and HAT. For a fair comparison, considering that some methods use the RRDB as the backbone and propose new training strategies or degradation models, we use the publicly available best models on the official code for evaluation, including ESRGAN, ESRGAN-FS, GFSNet, BSRGAN, DASR, Real-ESRGAN, and HGGT. In addition, some methods cannot be retrained on our degradation models because they need the blur kernel of real LR images during training, which is unavailable in hybrid degradation scenes. To be fair, we use the publicly available best models on the official code for evaluation, including IKC and DAN. As shown in Tab. 1 in the main body, although existing SOTA SR networks (\emph{i.e.}, HAT, RRDB, and SwinIR) train in the same experimental environments as ours (\emph{e.g.}, degradation models, training times, batch size, loss functions), our proposed method significantly outperforms them on both LPIPS and PSNR metrics while also having the advantage of low computational complexity. This demonstrates that our proposed method can achieve better results while being more easily applied to real-world scenarios and computationally constrained environments.





% \section{More ablation studies}
% \label{More ablation studies}



% \begin{table*}[h]
% \centering
% \caption{Ablation experiments for each proposed novel convolution on the DGConv.}
% \begin{tabular}{c|cc}
% \hline
%                                        & PSNR     & LPIPS   \\ \hline
% w/o vanilla convolution                & 25.33475 & 0.32785 \\
% w/o center-surrounding gradient convolution convolution      & 25.24596 & 0.32745 \\
% w/o horizontal gradient convolution        & 25.25321 & 0.32858 \\
% w/o vertical gradient convolution        & 25.21836 & 0.32243 \\
% w/o center-surrounding aggregation convolution & 25.24730 & 0.32381 \\
% \textbf{DGConv}                              & \textbf{25.45996} & \textbf{0.31946} \\ \hline
% \end{tabular*}
% \label{tab:Ablation_on_ADAPConv}
% \end{table}


% \begin{table*}[h]
% \centering
% \caption{Ablation experiment of intermediate feature channels (fea\_c) in the DGPNet.}
% \begin{tabular}{c|cccc}
% \hline
%                  fea\_c              & PSNR     & LPIPS   & FLOPs    & Params \\ \hline
% 32 (DGPNet\_tiny)           & 25.37300 & 0.34514 & 80.917   & 0.978  \\
% 48            & 25.30212 & 0.32478 & 181.168 & 2.195 \\
% \textbf{64 (DGPNet)} & \textbf{25.45996} & \textbf{0.31946} & \textbf{321.284}  & \textbf{3.899 } \\ \hline
% \end{tabular}
% \label{tab:Ablation_on_DGPNet}
% \end{table*}


% Here, we provide more ablation experiments for each convolution on the DGConv, and the results are shown in Tab. \ref{tab:Ablation_on_ADAPConv}. We can observe that each proposed convolution plays a crucial role in the representation capacity of DGConv, which verifies the rationality and efficiency of the proposed DGConv. At the same time, this also inspires us to determine whether adding more new directional arrangement convolution will further improve the representation capacity of DGConv. In addition, we also provide the ablation experiment of intermediate feature channels (Feature\_channels) in the DGPNet, and the results are shown in Tab. \ref{tab:Ablation_on_DGPNet}. We can observe that the proposed DGPNet still performs well under different intermediate feature channels, demonstrating the efficiency and validity of the proposed AIIBlock in the DGPNet.


















% \section{Detail about comparison with existing methods in Parameter and FLOPs}
% \label{Detail about comparison with existing methods in Parameter and FLOPs}
% As described in the main body, our method achieves the best performance on the PSNR metric while also achieving the second-best performance on the LPIPS metric. Since the computation cost of the model is critical for the Real-SR method to apply in the real world, we use FLOPs and Parameters to compare the computational cost between different methods, as shown in Tab \ref{tab:FLOPsAndPara}. We can observe that our proposed method’s parameters account for only 18.8\% of HAT and 23.4\% of Real-ESRGAN, and our proposed method’s FLOPs account for only 30.1\% of HAT and 27.3\% of Real-ESRGAN. In addition, we also propose a tiny version of our network, DGPNet\_tiny, which accounts for only 7.8\% and 6.8\% of the FLOPs of HAT and Real-ESRGAN, respectively, and has achieved comparable performance. This demonstrates that our proposed method not only has the best performance but also has the advantage of being lightweight and having a low computational cost, making it better suited for real-scenario applications.


% \begin{table*}[h]
% \centering
% \small
% \caption{Comparison of FLOPs and Parameters. Our methods and existing methods with SOTA performance are marked as  {\color[HTML]{FF0000} \textbf{bold}} and \textbf{bold}.}


% \begin{tabular}{ccccccccc}
% \hline
%         & SRResNet & EDSR    & RRDB     & VDSR     & SiwnIR  & HAT      & ESRGAN   & ESRGAN-FS       \\ \hline
% FLOPs   & 166.000  & 130.000 & 1176.000 & 700.684  & 539.000 & \textbf{1037.423} & 1175.584 & 1175.584 \\
% Params  & 1.520    & 1.520   & 16.700   & 1.112    & 11.720  & \textbf{20.773}   & 16.698   & 16.698   \\ \hline
% GFSNet  & DAN      & IKC     & Real-ESRGAN  & BSRGAN   & DASR    & HGGT     & DGPNet\_tiny     & DGPNet    \\ \hline
% 515.686 & 1250.519 & 338.804 & \textbf{1175.584} & 1175.584 & 209.314 & 1176.000 &{\color[HTML]{FF0000} \textbf{80.917} }  & {\color[HTML]{FF0000} \textbf{321.284}}  \\
% 6.626   & 4.330    & 7.966   & \textbf{16.698}   & 16.698   & 7.248   & 16.700   & {\color[HTML]{FF0000} \textbf{0.978}}    & {\color[HTML]{FF0000} \textbf{3.899}}    \\ \hline
% \end{tabular}
% \label{tab:FLOPsAndPara}
% \end{table*}











% \section{The evidence of cost-free improvement of DGConv}
% \label{The evidence of cost-free improvement of DGConv}
% \begin{table*}[h]
% \centering
% \caption{The performance and computational cost of VC-based and DGConv-based baseline. Note that VC-based and DGConv-based methods are marked as bold and \textbf{bold*}.}
% \begin{tabular}{c|cccc}
% \hline
% \multicolumn{1}{c|}{Methods} & PSNR\uparrow            & LPIPS\downarrow          & FLOPs(G)        & Params(M)        \\ \hline
% SRResNet                     & 24.996          & 0.352          & 166          & 1.52          \\
% \rowcolor[HTML]{C0C0C0} 
% \textbf{SRResNet*}           & \textbf{25.022} & \textbf{0.339} & \textbf{166} & \textbf{1.52} \\ \hline
% EDSR                         & 24.995          & 0.353          & 130          & 1.52          \\
% \rowcolor[HTML]{C0C0C0} 
% \textbf{EDSR*}               & \textbf{25.123} & \textbf{0.349} & \textbf{130} & \textbf{1.52} \\ \hline
% VDSR                         & 23.651          & 0.434          & 700          & 1.11          \\
% \rowcolor[HTML]{C0C0C0} 
% \textbf{VDSR*}               & \textbf{24.152} & \textbf{0.407} & \textbf{700} & 1.11          \\ \hline
% \end{tabular}
% \label{tab:cost_free}
% \end{table*}

% To further validate that our proposed DGConv can improve performance without introducing additional computational cost, we select three baselines (SRResNet, EDSR, and VDSR), train them using VC and DPConv, and compute their parameter and FLOPs. The results are shown in Tab. \ref{tab:cost_free}. We can observe that compared to the VC-based model, the DGConv-based model is able to improve both PSNR and LPIPS metrics, demonstrating the effectiveness of DGConv. Furthermore, we can observe that the computational cost (Params and FLOPs) of DGConv-based networks overhead is the same as that of VC-based networks. This demonstrates the superiority and lightweight properties of DGConv.








% \section{More detail about qualitative experimental results}
% \label{More detail about qualitative experimental results}

% Further, we compare with several sota and representative SR baselines, retrain them and our method on our train dataset with the same experimental setting, and directly evaluate the real-world test dataset proposed by \cite{cai2019toward}. The result is shown in Table \ref{tab:iccv2019_realSR}. We can observe that compared with representative SR methods, our proposed approach achieves the best performance on test sets captured in real scenarios.

% \begin{table}[h]

% \caption{The LPIPS and PSNS performance of test datasets \cite{cai2019toward}.}
% \centering
% % \scriptsize

% \begin{tabular}{c|cccccc}
% \hline
% Method & SRResnet & {VDSR} & EDSR   & {RRDB} & SwinIR & {Our} \\ \hline
% Canon-PSNR           & 26.741   & 25.731        & 26.343 & 26.244        & 26.679 & \textbf{27.167}       \\
% Canon-LPIPS          & 0.297    & 0.356         & 0.323  & 0.308         & 0.297  & \textbf{0.272}        \\ \hline
% Nikon-PSNR           & 25.742   & 24.696        & 25.558 & 25.325        & 25.849 & \textbf{26.432}       \\
% Nikon-LPIPS          & 0.321    & 0.378         & 0.345  & 0.337         & 0.314  & \textbf{0.295}        \\ \hline
% \end{tabular}


% \label{tab:iccv2019_realSR}
% \end{table}









% \section{Analysis of the kernel size of DGConv}
% \label{Analysis of the kernel size of DGConv}
% % Inspired by the edge extraction operators ( Sobel and Laplacian ) in traditional image processing and analyzing the imaging process of different types of degradation, we combine the learnable CNN and these operators, propose learnable center-surrounding gradient, center-surrounding aggregation, horizontal gradient, and vertical gradient convolutions to perceive degradation representations of direction arrangements adaptively. Since the size of the widely used Sobel and Laplacian operators and the widely used and cost-effective CNN size in deep learning networks are 3x3, the DGConv kernel size is empirically set to 3x3. In the future, we will consider extending DGConv to different scales to learn the representation of the large receptive field.

% Considering the widely-used kernel size in image super-resolution tasks and cost-effective CNNs is $3 \times 3$, we empirically set the DGConv kernel size to $3 \times 3$ to capture image details and degradation representation in this paper. 

% In the future, we will consider extending DGConv to different scales to learn representations of various receptive fields.


% \section{Reasons for using local mean in center-surrounding gradient and center-surrounding aggregation convolutions}
% \label{Reasons for using local mean in center-surrounding gradient and center-surrounding aggregation convolutions}
% Directly using values in the central location in our learnable center-surrounding gradient and center-surrounding aggregation convolutions ignores the most critical center-directional gradient and also may be challenging to capture all noise when the value of the central noise and the value of the surrounding noise are similar. To address this issue, we propose using the local mean as a gradient reference to capture diverse directional gradients. This can alleviate these problems and provide nine directional gradient arrangement information extending from the periphery to the center for representation learning.

% For center-surrounding aggregation convolutions, our design aims to capture local contrast statistics ( \emph{i.e.}, low-frequency statistical properties ). Using the value at the central position as the statistical property will inevitably introduce errors. Therefore, we propose directly using the mean component of the local statistical features to avoid these errors. To this end, we add the local mean to strengthen the proportion of statistical information and propose a learnable center-surrounding aggregation convolution to recover the statistical properties of images.

% To demonstrate the effectiveness of using the local mean in DGConv, we also conduct ablation experiments comparing the use of the local mean and the central value in our convolutions. We replace the local mean with the central value to generate DGConv* and test it on VDSR and EDSR baselines. The results are shown in the table below. We observe that the performance of DGConv decreased after replacing the local mean with the central value, which confirms the rationality and superiority of using the local mean in DGConv.

% % In traditional image processing, Laplacian uses the central value as the minus to calculate the gradient of eight field directions as the representation. However, this ignores the most critical center-directional gradient, and it is difficult to capture all noise when the noise values of the center and around are close. To this end, we propose to use the local mean as a gradient object, which can alleviate the above problems and provide nice directional gradient arrangement information extending from the periphery to the center for representation learning.

% % For center-surrounding aggregation convolutions, it is designed to capture local contrast statistics, \emph{i.e.} low-frequency statistics property. Therefore, using local mean and original response can be used to better perceive local contrast statistics.

% % At the same time, to prove the rationality of using local mean, we also conduct ablation experiments on local mean and central value in our convolutions. We replace the local mean with the central value to generate DGConv* and test on VDSR and EDSR baseline, and the results are shown in the table below. We can observe that the performance of DGConv decrease after using the center value instead of the local mean, which proves the rationality and superiority of using the local mean in DGConv.


% \begin{table*}[h]
% \centering
% \caption{Ablation experiment on the local mean. All represent the average performance of all scenarios. }
% \begin{tabular}{cc|cc|cc}
% \hline
% \multicolumn{2}{c|}{\multirow{2}{*}{methods}} & \multicolumn{2}{c|}{{VDSR}} & \multicolumn{2}{c}{{EDSR}} \\ \cline{3-6} 
% \multicolumn{2}{c|}{}                         & DGPConv         & DGPConv*         & DGPConv         & DGPConv*        \\ \hline
% \multirow{2}{*}{All}          & PSNR\uparrow          & 24.1525         & 24.0185          & 24.9949         & 24.7542         \\
%                               & LPIPS\downarrow         & 0.4068          & 0.4126           & 0.3532          & 0.3695          \\ \hline
% \end{tabular}
% \label{tab:1}
% \end{table*}





% \section{Sample visualizations of test data set}
% \label{Sample visualizations of test data set}
% \begin{figure*}[h]
%     \centering
%     \includegraphics[width=1.0\linewidth]{Fig/test_Datasets_sample.pdf}
%     \caption{Sample visualizations of test data set from Level I to Level V.}

%     \label{fig:Sample}
% \end{figure*}

% As demonstrated in the main body, we synthesize 500 real low-resolution and high-resolution image pairs by applying five different levels of degradation for evaluation. We provide examples of test data sets of different degradation levels, as shown in Fig \ref{fig:Sample}.


% \section{Feature visualization}
% \label{Feature visualization}
% To demonstrate that our proposed learnable center-surrounding gradient, horizontal gradient, and vertical gradient convolutions can extract directional gradients and our proposed learnable center-surrounding aggregation convolutions can extract image statistical properties, we choose SRResNet as the baseline to show their feature visualization results, as shown in Fig. \ref{fig:feature1} and Fig. \ref{fig:feature2}.

% We can see that the learnable horizontal gradient and vertical gradient convolutions can perceive horizontal and vertical directional gradient information, respectively. The learnable center-surrounding gradient convolution can extract directional gradient features in multiple directions, and the learnable center-surrounding aggregation convolution can extract image statistical properties (\emph{i.e.}, brightness distribution information). 


% \begin{figure*}[h]
%     \centering
%     \includegraphics[width=1.0\linewidth]{Fig/feature_vis2.png}
%     \caption{Feature visualization.}
%     \label{fig:feature1}
% \end{figure*}


% \begin{figure*}[h]
%     \centering
%     \includegraphics[width=1.0\linewidth]{Fig/feature_vis.png}
%     \caption{Feature visualization.}

%     \label{fig:feature2}
% \end{figure*}
